# Supplementary material for: Sublinear Time Algorithm for Online Weighted Bipartite Matching
Source: arXiv:2208.03367 source file (2024-02-12)
Supplement: Supplementary file 1 [file appendix.tex]

\section{Trash}

\subsection{Summary of \cite{cn20} and \cite{cn22}}

\begin{table}[H]

\begin{tabular}{|l|l|l|l|}
\hline
{\bf Ref} & {\bf Init} & {\bf Query}  &{\bf Update}\\ \hline
\cite{cn20} &$O(\epsilon^{-2}nd(d+\log(1/\delta)))$ & $O(\epsilon^{-2}(n+d)\log(n/\delta))$ &  $O(\epsilon^{-2}d(d+\log(1/\delta)))$  \\ \hline
\cite{cn22} &  $\tilde{O}(\epsilon^{-2} nd \log(1/\delta))$ &  $\tilde{O}(\epsilon^{-2}(n+d)\log(1/\delta))$ &  $\tilde{O}(\epsilon^{-2} d \log(1/\delta))$               \\ \hline 
\end{tabular}

\caption{$\epsilon$ denotes the accuracy parameter. $\delta$ denotes the failure probability. $n$ denotes the number of data points. $d$ denotes the data point dimension. }
\end{table}

\begin{table}[H]

\begin{tabular}{|l|l|l|l|l|}
\hline
{\bf Refs}   & {\bf Space} & {\bf Sketch Size} &  \#{\bf Sketches} & \#{\bf  Samples} \\ \hline
\cite{cn20} 
& $O(\epsilon^{-2}(n+d)(d+\log(1/\delta)))$ 
& $\Theta(\epsilon^{-2})$        
& $\Theta(d + \log(1/\delta))$           
&  $\Theta(\log(n /\delta))$            \\ \hline
\cite{cn22}     
&  $O(\epsilon^{-2}nd \log(1/\delta) )$
&  $\Theta(d)$  
&  $\tilde{\Omega}(\epsilon^{-2} \log(1/\delta) )$       
&  $\tilde{\Omega}(\epsilon^{-2} \log(1/\delta))$       \\ \hline  
\end{tabular}

\caption{$\epsilon$ denotes the accuracy parameter. $\delta$ denotes the failure probability. $n$ denotes the number of data points. $d$ denotes the data point dimension.  }
\end{table}
